# Supplementary material for: A Matrix Autoencoder Framework to Align the Functional and Structural Connectivity Manifolds as Guided by Behavioral Phenotypes
Source: arXiv:2105.14409 source file (2021-07-09)
Supplement: Supplementary file 1 [file MICCAI_2021_Supplementary.pdf]

# Supplementary Results

***

***

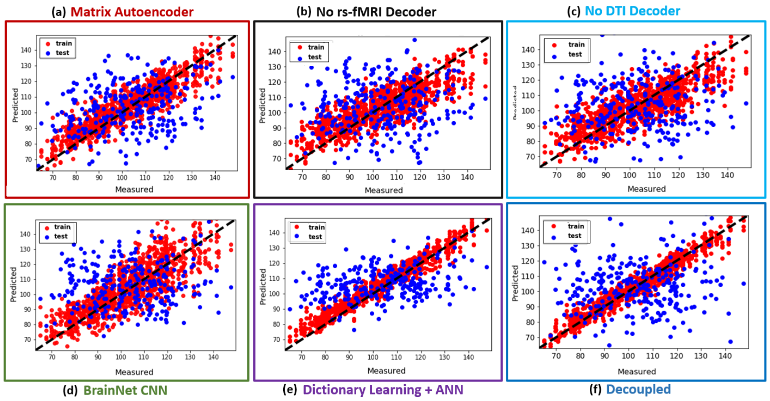


**Fig. 1. HCP Dataset** Prediction of CFIS by **(a)** Our Framework **(b)** Matrix AE without rs-fMRI Decoder **(c)** Matrix AE without DTI Decoder **(d)** BrainNet CNN **(e)** Dictionary Learning + ANN **(f)** Decoupled Matrix AE and ANN

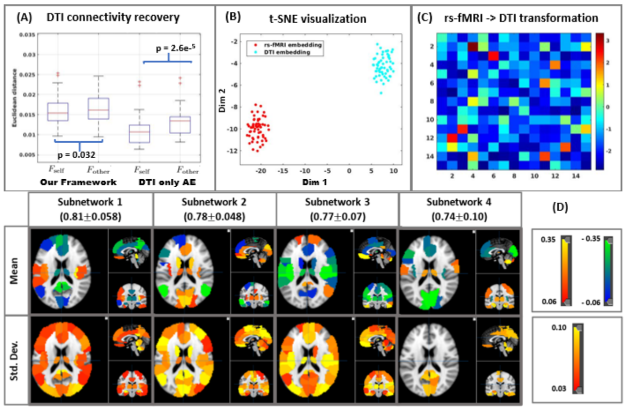


**Fig. 2. ASD Dataset: (A)** Recovery of SC by **(L):** Our Framework **(R):** DTI only AE **(B)** t-SNE visualization of FC and SC embeddings **(C)** Coeff. of Var. ($C_v$) (log scale) for $\mathbf{\Phi}_{\text{align}}(\cdot)$ weights. Cold colors imply better stability **(D)** Top four FC bases

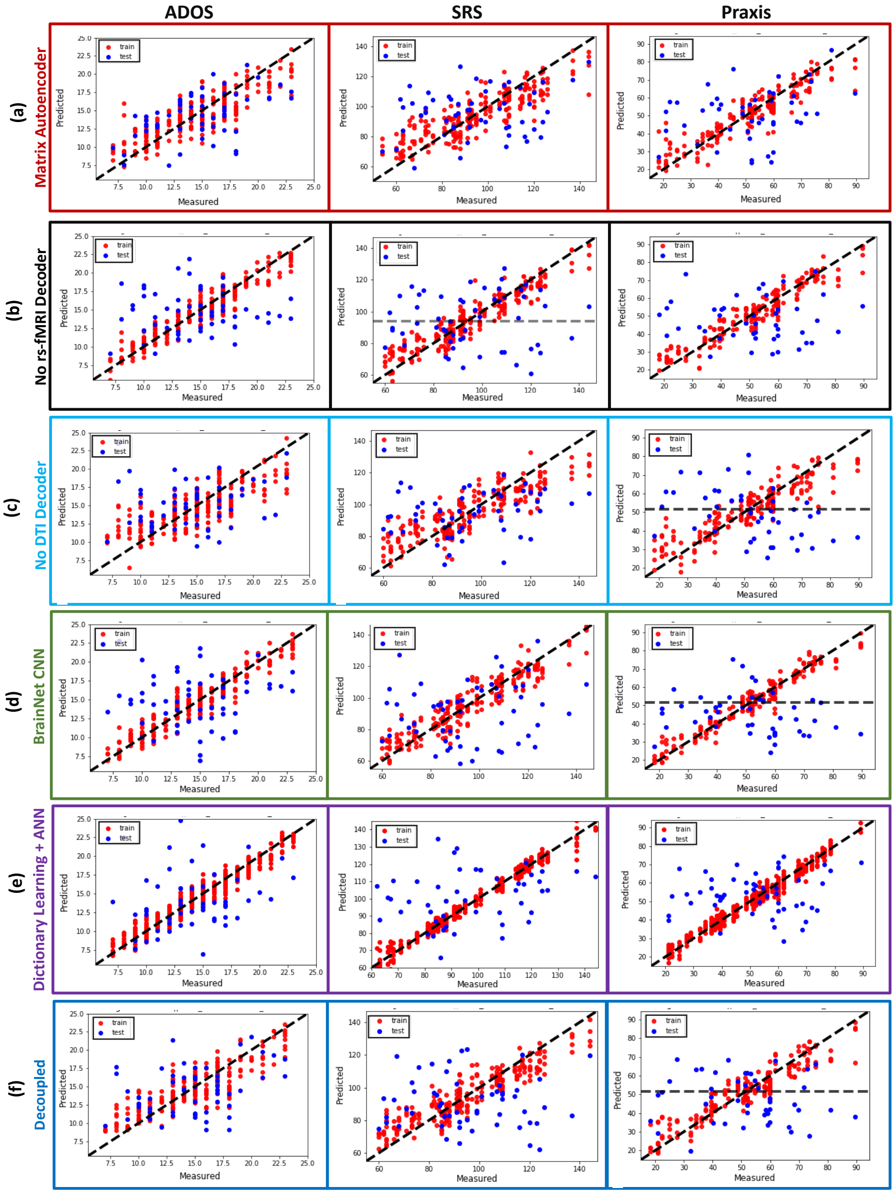


**Fig. 3. ASD Dataset:** Multi-output prediction performance of **(L):** ADOS **(M):** SRS **(R):** Praxis by **(a)** Our Framework **(b)** Matrix Autoencoder without rs-fMRI Decoder **(c)** Matrix Autoencoder without DTI Decoder **(d)** BrainNet CNN **(e)** Dictionary Learning + ANN **(f)** Decoupled Matrix Autoencoder and ANN
